# Supplementary material for: Decomposing causality into its synergistic, unique, and redundant components
Source: arXiv:2405.12411 source file (2024-08-21)
Supplement: Supplementary file 2 [file logistic_map_12_intermediate_123_uncoupled.tex]

% \documentclass[class=scrreprt]{standalone}
% \usepackage[utf8]{inputenc}
% \usepackage[T1]{fontenc}
% \usepackage{lmodern}
% \usepackage{tikz}
% \usetikzlibrary{decorations.pathmorphing,arrows.meta}
% \definecolor{myc1}{HTML}{003049}
% \definecolor{myc2}{HTML}{d62828}
% \definecolor{myc3}{HTML}{f77f00}
% \definecolor{myc4}{HTML}{6ca13b}

% \begin{document}

\begin{tikzpicture}[cir/.style={circle,draw=black!70!white,,thick,inner sep=.5em},
    >={Latex[length=.2cm]},scale=.8]
    
    % \colorlet{cA}{myc2!30!white}
    % \colorlet{cB}{myc1!30!white}
    % \colorlet{cC}{myc3!30!white}

    \colorlet{cA}{Q1!30!white}
    \colorlet{cB}{Q2!30!white}
    \colorlet{cC}{Q3!30!white}

    % \colorlet{cA}{black!5}
    % \colorlet{cB}{black!5}
    % \colorlet{cC}{black!5}

    \node [cir,fill=cB] (q1) at (-1,+1)   {$Q_1$}; 
    \node [cir,fill=cA] (q2) at (-1,-1)   {$Q_2$}; 
    \node [cir,fill=cC] (q3) at (+0.73,0)    {$Q_3$}; 
    
    % \node [anchor=north] at (q2.south) {\scriptsize mediator};

    % \draw[decorate,decoration={snake,post length=4pt,amplitude=.2em}, thick,->]
    % (-2.3,1) node[anchor=east] {$W_3$} -- (q3);
    % \draw[decorate,decoration={snake,post length=4pt,amplitude=.2em}, thick,->]
    % (-2.3,-1) node[anchor=east] {$W_2$} -- (q2);
    % \draw[decorate,decoration={snake,post length=4pt,amplitude=.2em}, thick,->]
    % (.73,-1.3) node[anchor=north] {$W_1$} -- (q1);

    \path[thick,->]%[every node/.style={font=\sffamily\small}]
        (q1) edge[bend right] node [left] {} (q2);
        % (q2) edge[bend right] node [left] {} (q1);
    \path[thick,<-] (q3) edge[loop right] node {} (q3);
    \path[thick,<-] (q2) edge[loop below] node {} (q2);
    \path[thick,<-] (q1) edge[loop above] node {} (q1);
    
\end{tikzpicture}

% \end{document}
