# Supplementary material for: Decomposing causality into its synergistic, unique, and redundant components
Source: arXiv:2405.12411 source file (2024-08-21)
Supplement: Supplementary file 7 [file moran_effect.tex]

% \documentclass[class=scrreprt]{standalone}
% \usepackage[utf8]{inputenc}
% \usepackage[T1]{fontenc}
% \usepackage{lmodern}
% \usepackage{tikz}
% \usetikzlibrary{decorations.pathmorphing,arrows.meta}
% \definecolor{myc1}{HTML}{003049}
% \definecolor{myc2}{HTML}{d62828}
% \definecolor{myc3}{HTML}{f77f00}
% \definecolor{myc4}{HTML}{6ca13b}

% \begin{document}

\begin{tikzpicture}[cir/.style={circle,draw=black!70!white,,thick,inner sep=.5em},
    >={Latex[length=.2cm]},scale=0.9]
    
    \colorlet{cA}{myc2!30!white}
    \colorlet{cB}{myc1!30!white}
    \colorlet{cC}{myc3!30!white}

    \node [cir,fill=cB] (V) at (-3,0) {$V$}; 

    \node [cir,fill=cA] (R2) at (-1,-1) {$R_2$}; 
    \node [cir,fill=cA] (R1) at (-1,+1) {$R_1$}; 

    \node [cir,fill=cC] (N2) at (1,-1) {$N_2$}; 
    \node [cir,fill=cC] (N1) at (1,+1) {$N_1$}; 

    % \node [anchor=west] at (q3.north) {\quad \scriptsize confounder};

    \path[thick,->]%[every node/.style={font=\sffamily\small}]
        (V) edge[bend left] node [right] {} (R1)
        (V) edge[bend right] node [left] {} (R2);
    \path[thick,<->] (R1) edge[right] node {} (N1);
    \path[thick,<->] (R2) edge[right] node {} (N2);
    % \path[thick,<-] (q2) edge[loop below] node {} (q2);
    % \path[thick,<-] (q3) edge[loop above] node {} (q3);

\end{tikzpicture}

% \end{document}
